# Supplementary material for: Precision and accuracy of single-molecule FRET measurements - a worldwide benchmark study
Source: arXiv:1710.03807 ancillary file (2017-12-29)
Supplement: Supplementary file 1 [file FRET_Comp_Suppl_rxv.pdf]

# **Supplementary Material:**

## **Precision and accuracy of single-molecule FRET measurements –**

### **a worldwide benchmark study**

Björn Hellenkamp<sup>1,°</sup>, Sonja Schmid<sup>1,°</sup>, Olga Doroshenko<sup>20</sup>, Oleg Opanasyuk<sup>20</sup>, Ralf Kühnemuth<sup>20</sup>, Soheila Rezaei Adariani<sup>15</sup>, Anders Barth<sup>21</sup>, Victoria Birkedal<sup>9</sup>, Mark E. Bowen<sup>11</sup>, Hongtao Chen<sup>26</sup>, Thorben Cordes<sup>14,25</sup>, Tobias Eilert<sup>19</sup>, Carel Fijen<sup>7</sup>, Markus Götz<sup>1</sup>, Giorgos Gouridis<sup>14,25</sup>, Enrico Gratton<sup>26</sup>, Taekjip Ha<sup>22</sup>, Christian A. Hanke<sup>20</sup>, Andreas Hartmann<sup>17</sup>, Jelle Hendrix<sup>5,6</sup>, Lasse L. Hildebrandt<sup>9</sup>, Johannes Hohlbein<sup>7,8</sup>, Christian G. Hübner<sup>16</sup>, Eleni Kallis<sup>19</sup>, Achillefs N. Kapanidis<sup>10</sup>, Jae-Yeol Kim<sup>23</sup>, Georg Krainer<sup>17,18</sup>, Don C. Lamb<sup>21</sup>, Nam Ki Lee<sup>23</sup>, Edward A. Lemke<sup>3</sup>, Brié Levesque<sup>11</sup>, Marcia Levitus<sup>24</sup>, James J. McCann<sup>11</sup>, Nikolaus Naredi-Rainer<sup>21</sup>, Daniel Nettels<sup>4</sup>, Thuy Ngo<sup>22</sup>, Ruoyi Qiu<sup>12</sup>, Carlheinz Röcker<sup>19</sup>, Hugo Sanabria<sup>15</sup>, Michael Schlierf<sup>17</sup>, Benjamin Schuler<sup>4</sup>, Henning Seidel<sup>16</sup>, Lisa Streit<sup>19</sup>, Philip Tinnefeld<sup>13,27</sup>, Swati Tyagi<sup>3</sup>, Niels Vandenberk<sup>5</sup>, Keith R. Weninger<sup>12</sup>, Bettina Wünsch<sup>13</sup>, Inna S. Yanez-Orozco<sup>15</sup>, Jens Michaelis<sup>19,\*</sup>, Claus A.M. Seidel<sup>20,\*</sup>, Timothy D. Craggs<sup>2,10,\*</sup>, Thorsten Hugel<sup>1,\*</sup>

<sup>1</sup>Institute of Physical Chemistry, University of Freiburg, Germany

<sup>2</sup>Department of Chemistry, University of Sheffield, S3 7HF, UK

<sup>3</sup>Structural and Computational Biology Unit, EMBL Heidelberg, Germany

<sup>4</sup>Department of Biochemistry, University of Zurich, Switzerland

<sup>5</sup>Laboratory for Photochemistry and Spectroscopy, Department of Chemistry, University of Leuven, B-3001 Leuven, Belgium

<sup>6</sup>Present address: Hasselt University, Faculty of Medicine and Life Sciences and Biomedical Research Institute, B-3590 Hasselt, Belgium

<sup>7</sup>Laboratory of Biophysics, Wageningen University & Research, 6708 WE, Wageningen, NL

<sup>8</sup>Microspectroscopy Research Facility Wageningen, Wageningen University & Research, 6708 WE, Wageningen, NL

<sup>9</sup>Interdisciplinary Nanoscience Center and Department of Chemistry, Aarhus University, 8000 Aarhus C, Denmark

<sup>10</sup>Gene Machines group, Clarendon Laboratory, Department of Physics, University of Oxford, Parks Road, OX1 3PU, Oxford, UK

<sup>11</sup>Department of Physiology & Biophysics, Stony Brook University, Stony Brook, NY 11794, USA

<sup>12</sup>Department of Physics, North Carolina State University, Raleigh, NC 27695 USA

<sup>13</sup>Institute of Physical & Theoretical Chemistry, and Braunschweig Integrated Centre of Systems Biology (BRICS), and Laboratory for Emerging Nanometrology (LENA), Braunschweig University of Technology, Rebenring 56, 38106 Braunschweig, Germany

<sup>14</sup>Molecular Microscopy Research Group, Zernike Institute for Advanced Materials, University of Groningen, Nijenborgh 4, 9747 AG Groningen, The Netherlands

<sup>15</sup>Department of Physics and Astronomy, Clemson University, 29634 Clemson, SC, USA

<sup>16</sup>Institute of Physics, University of Lübeck, Germany

<sup>17</sup>B CUBE – Center for Molecular Bioengineering, TU Dresden, Arnoldstr. 18, 01307 Dresden, Germany

<sup>18</sup>Molecular Biophysics, University of Kaiserslautern, Erwin-Schrödinger-Str. 13, 67663 Kaiserslautern, Germany.

<sup>19</sup>Institute for Biophysics, Ulm University, Albert-Einstein-Allee 11, 89081 Ulm, Germany

<sup>20</sup>Chair for Molecular Physical Chemistry, Heinrich-Heine-Universität Düsseldorf, 40225 Düsseldorf, Germany

<sup>21</sup>Lamb lab, Department of Chemistry, LMU Munich, Butenandtstrasse 5-13, 81377 Germany

<sup>22</sup>Ha lab, Department of Biomedical Engineering, John Hopkins University, USA

<sup>23</sup>School of Chemistry, Seoul National University, Seoul, South Korea

<sup>24</sup>School of Molecular Sciences and The Biodesign Institute, Arizona State University, USA

<sup>25</sup>Physical and Synthetic Biology, Faculty of Biology, Ludwig Maximilians-Universität München, Großhadernerstr. 2-4, 82152 Planegg-Martinsried, Germany

<sup>26</sup>Department of Biomedical Engineering, University of California, Irvine, Irvine, California, USA

<sup>27</sup>Department of Chemistry, Ludwig-Maximilians-Universitaet Muenchen, Butenandtstr. 5-13, 81377 München, Germany.

° these authors contributed equally

\* corresponding authors: jens.michaelis@uni-ulm.de; cseidel@hhu.de; t.craggs@sheffield.ac.uk; thorsten.hugel@pc.uni-freiburg.de

| <b>Supplementary Information</b>                                                                                                                                        | <b>Page</b> |
|-------------------------------------------------------------------------------------------------------------------------------------------------------------------------|-------------|
| <b>Supplementary Figure 1</b><br>Structural formula of the dyes used in this study                                                                                      | 3           |
| <b>Supplementary Figure 2</b><br>FRET efficiencies of all labs for all measured samples 1-4                                                                             | 4           |
| <b>Supplementary Figure 3</b><br>Schematics of a typical confocal setup with alternating laser excitation / pulsed interleaved excitation and color-sensitive detection | 5           |
| <b>Supplementary Figure 4</b><br>Schematic designs of an objective-type (a) and a prism-type TIRF setup                                                                 | 6           |
| <b>Supplementary Figure 5</b><br>Accounting for the differences in the excitation intensity profiles of the green and red laser across the field of view                | 7           |
| <b>Supplementary Figure 6</b><br>Computation of the spectral overlap integral J for the FRET pair Atto550-Atto647N in sample 1                                          | 8           |
| <b>Supplementary Figure 7</b><br>Visualizations of different averages for efficiencies according to different fluorophore dynamics.                                     | 9           |
| <b>Supplementary Figure 8</b><br>Time-resolved anisotropies and FRET                                                                                                    | 10          |
| <b>Supplementary Table 1</b><br>Spectroscopic parameters of the dyes in samples 1 and 2.                                                                                | 11          |
| <b>Supplementary Note 1:</b><br>Time-resolved experiments                                                                                                               | 13          |
| <b>Supplementary Note 2</b><br>AV simulations to compute donor acceptor distances                                                                                       | 18          |
| <b>Supplementary Note 3</b><br>$R_E$ to $R_{MP}$ conversion                                                                                                             | 19          |
| <b>Supplementary Note 4</b><br>Error propagation                                                                                                                        | 22          |
| <b>Supplementary Note 5</b><br>Further samples                                                                                                                          | 23          |
| <b>Supplementary Note 6</b><br>MD simulations                                                                                                                           | 24          |
| <b>Biobibliography</b>                                                                                                                                                  | 27          |

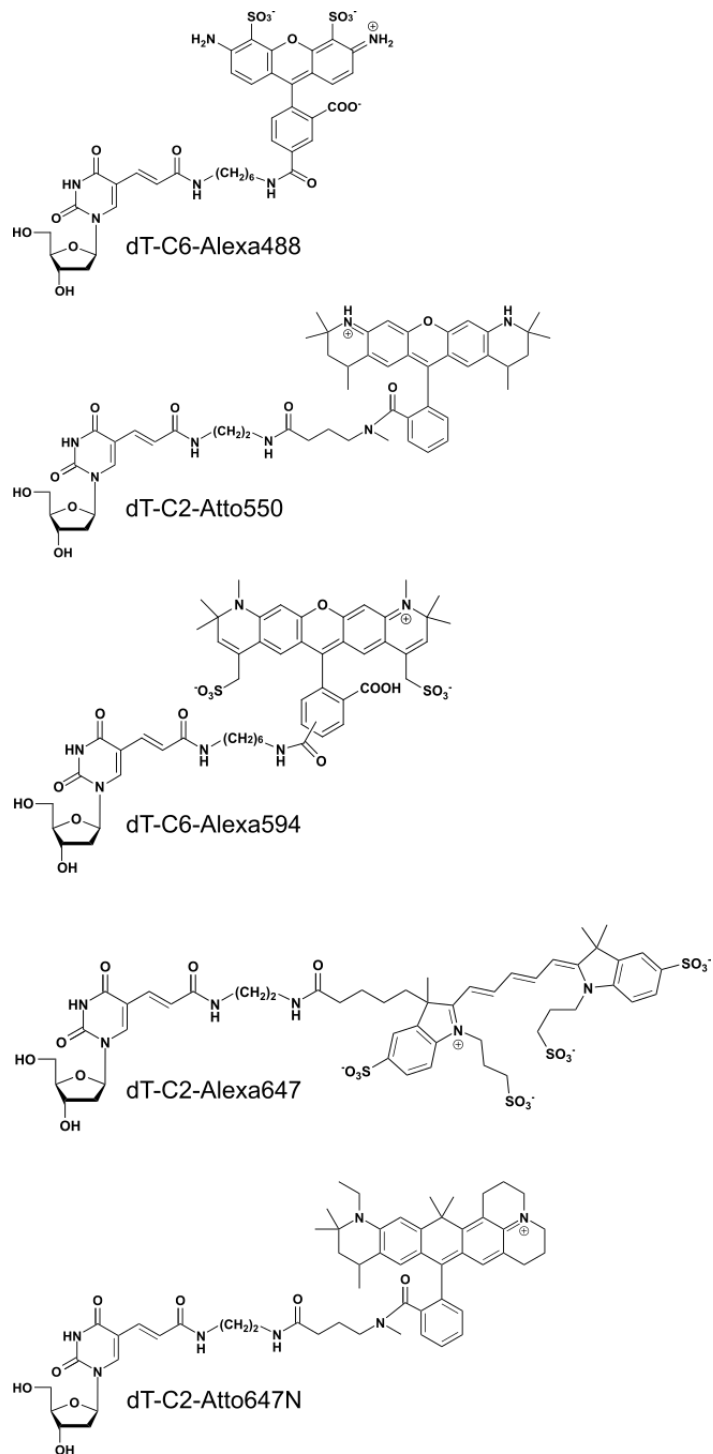

**Supplementary Figure 1:** Structural formula of the dyes used in this study. Based on dyes from Molecular Probes / Thermo Fisher Scientific (Waltham, USA) and Atto-tec (Siegen, D).

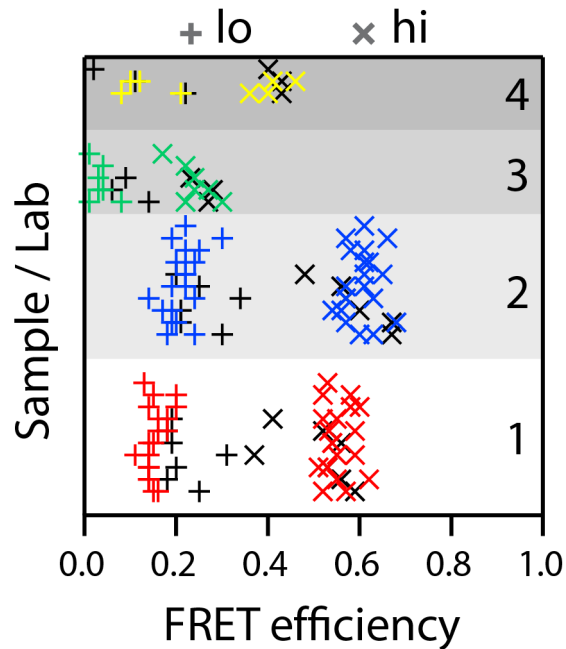

**Supplementary Figure 2:** FRET efficiencies of all labs for all measured samples as indicated. Sample 1 to 4 (see Table 5 and Supplementary Note 5) are color coded (red, blue, green, yellow) for all data points from intensity-based techniques. For a table of  $R_{E_i}$  and  $R_{MP}$  see Table 4 (main text). Ensemble lifetime, single molecule lifetime and phasor approach derived data is shown in black. The FRET efficiencies (means and s.d.) for these measurements (depicted in black) are:  $E_{1a}=0.21\pm0.05$ ;  $E_{1b}=0.51\pm0.08$ ;  $E_{2a}=0.25\pm0.06$ ;  $E_{2b}=0.59\pm0.07$ ;  $E_{3a}=0.10\pm0.04$ ;  $E_{3b}=0.26\pm0.03$ ;  $E_{4a}=0.12\pm0.10$ ;  $E_{4b}=0.42\pm0.02$ .

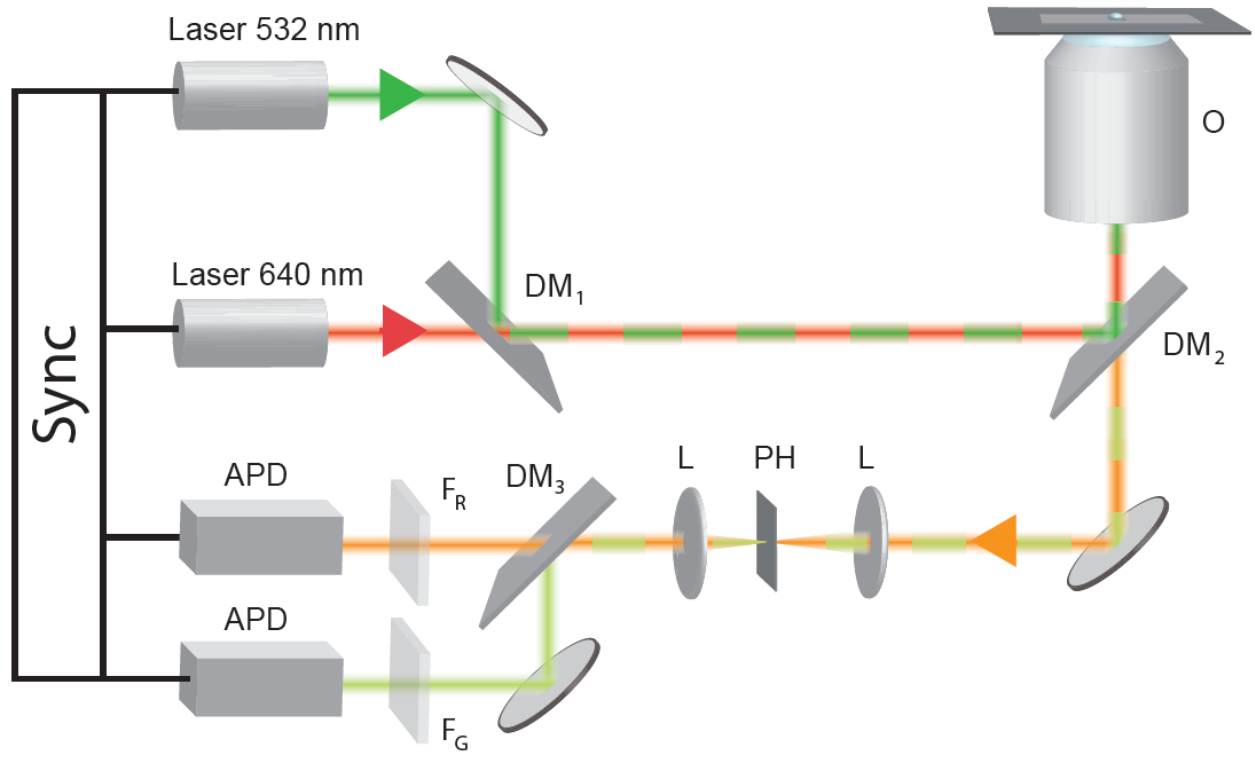

**Supplementary Figure 3:** Schematics of a typical confocal setup with alternating laser excitation / pulsed interleaved excitation and color-sensitive detection. The most important elements are specified: Objective (O), dichroic mirror (DM), pinhole (P), spectral filter (F), avalanche photo diode (APD) and electronic micro- or picosecond synchronization of laser pulses and single photon counting (Sync).

Elements used for the correction factors in Table 2 (main text) were: F34-641 Laser Clean-up Filter z 640/10 (right after Laser 640 nm); DM<sub>1</sub>: F43-537 Laser-Strahlenteiler z 532 RDC ; DM<sub>2</sub>: F53-534 Dual Line Strahlenteiler z 532/633; DM<sub>3</sub>: F33-647 Laser-Strahlenteiler 640 DCXR; F<sub>G</sub>: F37-582 Brightline HC 582/75; F<sub>R</sub>: F47-700 ET Bandpass 700/75; Objective: Cfi plan apo VC 60xWI, NA1.2; Detectors: MPD picoquant (green), tau-SPAD, picoquant (red); Pinholes: 100  $\mu\text{m}$ ; ; Laser power at sample:  $\approx 100 \mu\text{W}$ ; Beam diameter  $\approx 2\text{mm}$ ; Diffusion time of Atto550 and Atto647N around 0.42 ms and 0.50 ms, respectively.

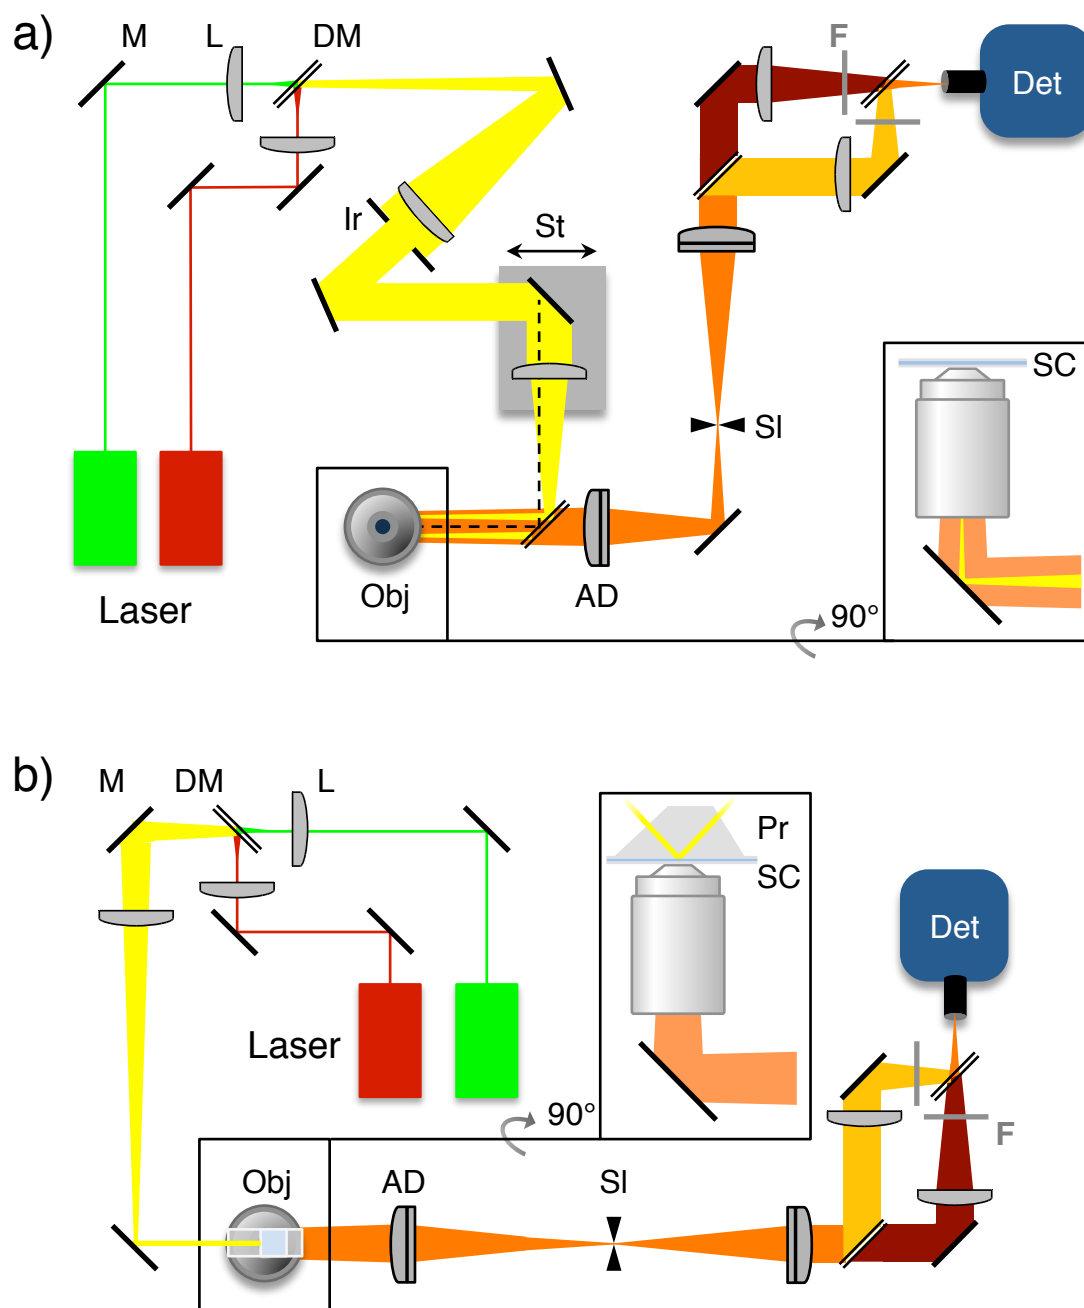

**Supplementary Figure 4:** Schematic designs of an objective-type (a) and a prism-type TIRF setup (b). Green and red lasers are used to excite donor and acceptor dyes, respectively. M, mirror. L, lens. DM, dichroic mirror. Obj, objective. AD, achromatic doublet lens. Sl, tunable slit. F, filters. Det, detector (e.g. electron multiplying charge-coupled device camera, EMCCD). The inset shows a side view of the objective with the out-of-plane ( $45^\circ$ ) mirror below. SC, sample chamber. Ir, iris. St, translation stage, Pr, prism. The dashed black line in (a) indicates the *on-axis* path to the objective, in contrast to the displayed *off-axis* path for TIR illumination. Elements used for the correction factors in Table 2 (main text) were: Dichroic before objective: F53-534 (AHF), Dichroics in detection: F33-726 and F33-644 (AHF). Band pass filters in detection: BP F39-572 and BP F37-677 (AHF). SI: SP40 (Owis), Objective: CFI Apo TIRF 100x, NA 1.49 (Nikon). Camera: EMCCD, iXonUltra, Andor. Lasers: 532nm, Compass 215M (Coherent) and 635nm, Lasiris (Stoker Yale).

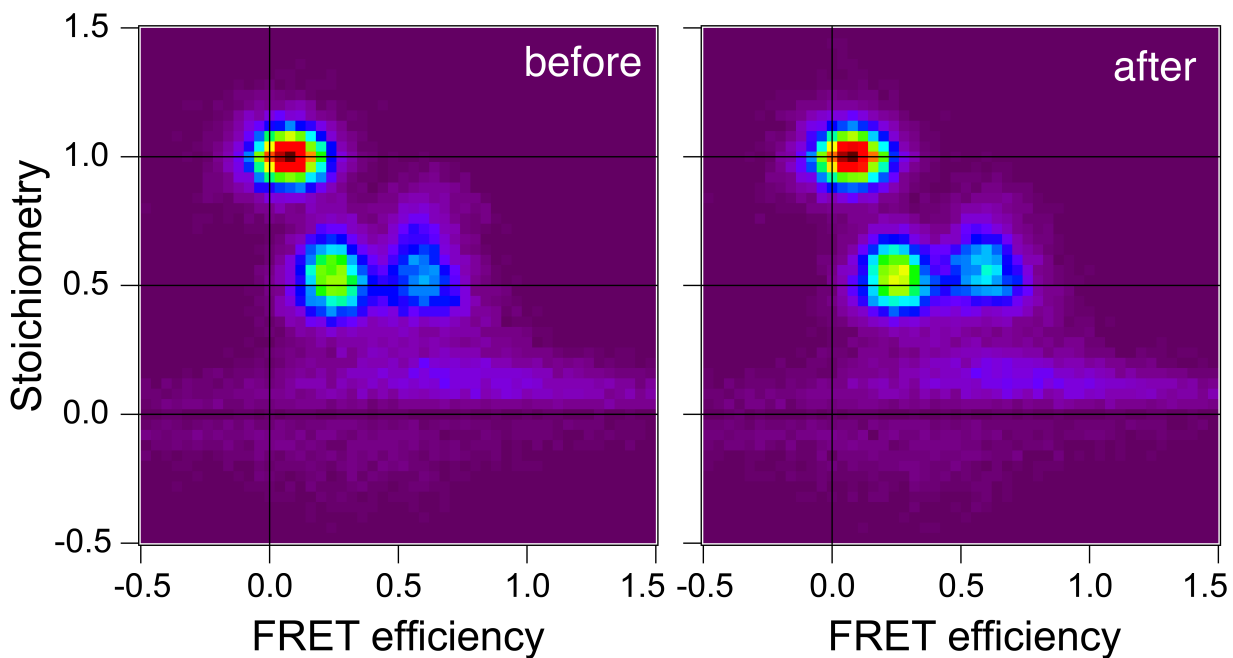

**Supplementary Figure 5:** Accounting for the differences in the excitation intensity profiles of the green and red laser across the field of view. The individual excitation profiles are determined as the mean image of a stack of images recorded while moving across a dense layer of dyes. In contrast to the uncorrected case (“before”), a position specific normalization creates narrower and more symmetric SE-populations (“after”). The standard corrections described in the main text are performed subsequently.

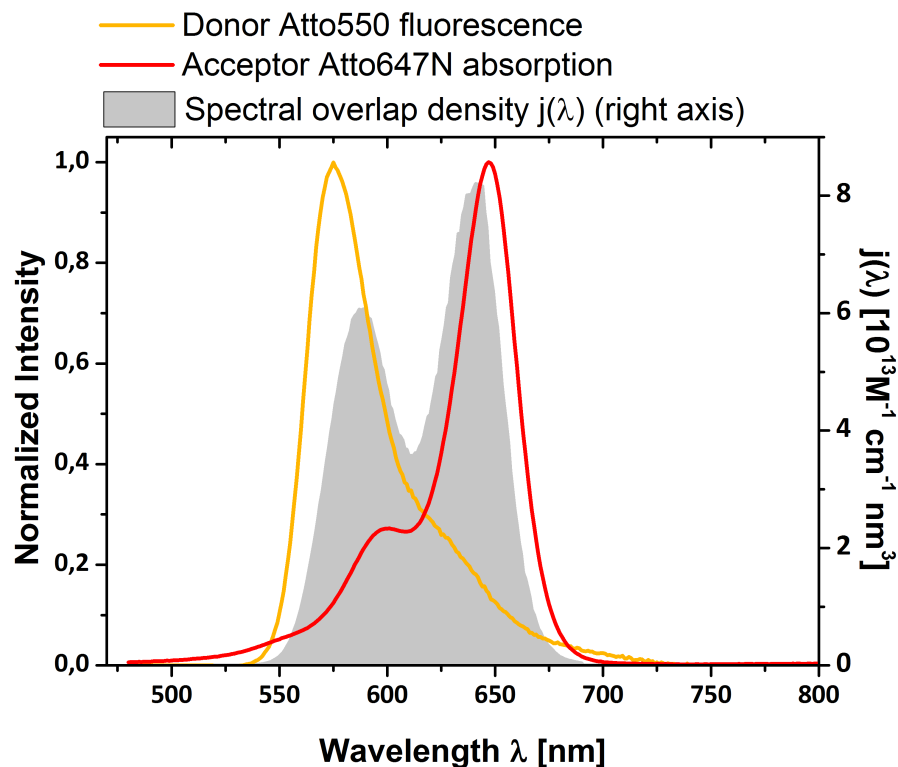

**Supplementary Figure 6:** Computation of the spectral overlap integral  $J$  for the FRET pair Atto550-Atto647N in sample 1. Normalized donor fluorescence and acceptor absorption spectra normalized to the maximum (left scale). Spectral overlap density  $j(\lambda)$  (right scale) to compute the spectral overlap integral  $J$  [ $\text{cm}^{-1} \text{ M}^{-1} \text{ nm}^4$ ] with  $J = \int_0^\infty j(\lambda) d\lambda$  and  $j(\lambda) = \bar{F}_D(\lambda) \varepsilon_A(\lambda) \lambda^4$ . The extinction coefficient  $\varepsilon_A$  of Atto647N was assumed to be  $150000 \text{ M}^{-1} \text{ cm}^{-1}$  at the maximum as provided by the manufacturer.



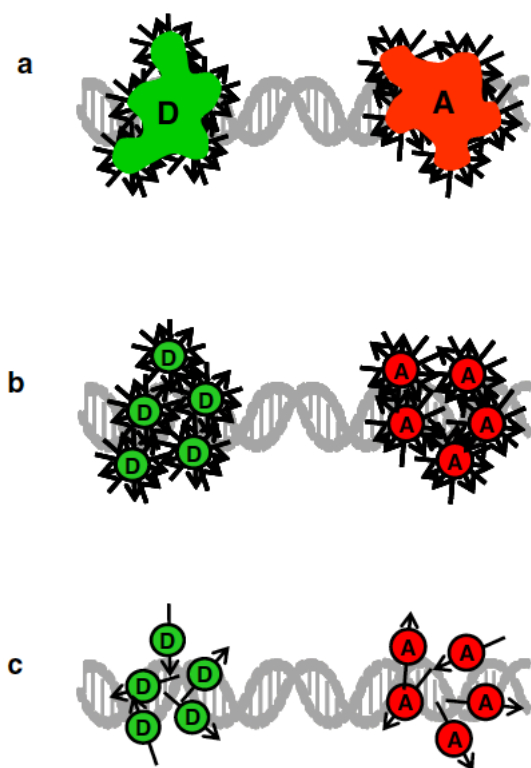

**Supplementary Figure 7:** Visualizations of different averages for efficiencies according to different fluorophore dynamics. (a) Dynamic average, which applies in the case of the fluorophore movements being faster than the rate of energy transfer. There the rate of energy transfer has to be calculated taking into account the average over all possible distances and orientations. (b) Intermediate case, called the isotropic average, where the orientational variation of the fluorophores is faster than the rate of energy transfer while the positional variation is slower (c) Static case, where the fluorophore movements are much slower than the rate of energy transfer. In this case each distance and respective fluorophore orientation has to be taken into account with its individual transfer efficiency. These efficiencies then are averaged by the measurement process. (Figure from ref. <sup>1</sup>).

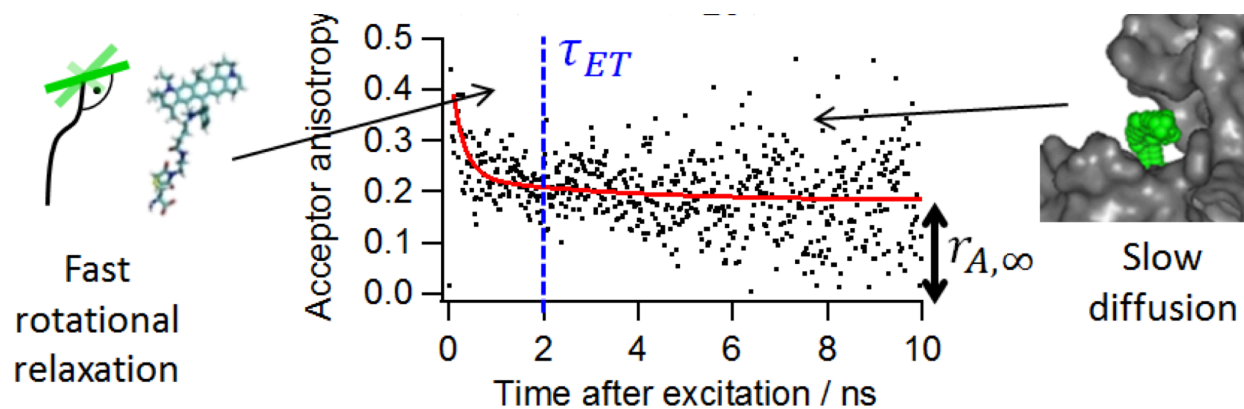

**Supplementary Figure 8:** Time-resolved anisotropies and FRET. The time-resolved anisotropies of dyes bound to a larger object (e.g. DNA or protein) normally consist of a fast decay from rotational relaxation of the dipole (left) and of a slow decay from translational relaxation (right).  $\tau_{ET} = 1/k_{FRET}$ : time of energy transfer;  $r_{A,\infty}$ : residual anisotropy of dye A. (Figure from ref. <sup>2</sup>)

**Supplementary Table 1:** Spectroscopic parameters of the dyes in samples 1 and 2. Residual anisotropy  $r_\infty$ , combined anisotropy  $r_c$ , fluorescence quantum yields of donor and acceptor  $\Phi_{F,D}$  and  $\Phi_{F,A}$ , respectively (determined according to the procedure detailed in the online methods), and species average fluorescence lifetimes  $\langle\tau\rangle_x$  for the samples 1 (Atto550 /Atto647N) and the samples 2 (Atto550 /Alexa647). All measurements were done in 20mM MgCl<sub>2</sub>, 5mM NaCl, 5mM TRIS at pH 7.5 measurement buffer.

| <b>Sample 1</b>                                             | <b>1-lo(Atto550)</b>  | <b>1-lo (Atto647N)</b> | <b>1-hi (Atto550)</b> | <b>1-hi (Atto647N)</b> |
|-------------------------------------------------------------|-----------------------|------------------------|-----------------------|------------------------|
| Base position (Linker), strand                              | T 31, (C2), D-strand  | T 31(C2), A-strand     | T 23(C2), D-strand    | T 31(C2), A-strand     |
| Residual anisotropy $r_{A,\infty}$ or $r_{D,\infty}$ [a]    | 0.08                  | 0.07                   | 0.11                  | 0.07                   |
| Combined anisotropy $r_c$                                   | 0.07                  |                        | 0.09                  |                        |
| Steady state anisotropy $r_S$                               | 0.11                  | 0.09                   | 0.13                  | 0.09                   |
| Lifetime $\langle\tau\rangle_x$ / ns (SD: 2%) [b]           | 3.76                  | 3.62                   | 3.81                  | 3.62                   |
| Fluorescence quantum yield $\Phi_{F,D}$ or $\Phi_{F,A}$     | 0.77±0.015[c]         | 0.65 [d]               | 0.77±0.015[c]         | 0.65 [d]               |
| $R_\theta$ [Å] [e]                                          | 62.6                  |                        |                       |                        |
| $\langle\Phi_{F,D}\rangle$ [e]                              | 0.765                 |                        |                       |                        |
| $\epsilon_A$ [M <sup>-1</sup> cm <sup>-1</sup> ]            | 150000                |                        |                       |                        |
| $J$ [cm <sup>-1</sup> nm <sup>4</sup> M <sup>-1</sup> ]     | $5.180 \cdot 10^{15}$ |                        |                       |                        |
| $n_{im}$                                                    | 1.40                  |                        |                       |                        |
| $\kappa^2$                                                  | 2/3                   |                        |                       |                        |
| <b>Sample 2</b>                                             | <b>2-lo(Atto550)</b>  | <b>2-lo (Alexa647)</b> | <b>2-hi (Atto550)</b> | <b>2-hi (Alexa647)</b> |
| Base position (Linker), strand                              | T 31, (C2), D-strand  | T 31(C2), A-strand     | T 23(C2), D-strand    | T 31(C2), A-strand     |
| Residual anisotropy $r_{A,\infty}$ or $r_{D,\infty}$ [a]    | 0.08                  | 0.05                   | 0.11                  | 0.05                   |
| Combined anisotropy $r_c$                                   | 0.06                  |                        | 0.07                  |                        |
| Steady state anisotropy $r_S$                               | 0.11                  | 0.15                   | 0.14                  | 0.14                   |
| Lifetime $\langle\tau\rangle_x$ / ns (SD: 2%) [b]           | 3.76                  | 1.19                   | 3.81                  | 1.19                   |
| Fluorescence quantum yield $\Phi_{F,D}$ or $\Phi_{F,A}$ [c] | 0.77±0.015[c]         | 0.35                   | 0.77±0.015[c]         | 0.35                   |
| $R_\theta$ [Å] [e]                                          | 68.0                  |                        |                       |                        |
| $\langle\Phi_{F,D}\rangle$ [e]                              | 0.765                 |                        |                       |                        |
| $\epsilon_A$ [M <sup>-1</sup> cm <sup>-1</sup> ]            | 270000                |                        |                       |                        |
| $J$ [cm <sup>-1</sup> nm <sup>4</sup> M <sup>-1</sup> ]     | $8.502 \cdot 10^{15}$ |                        |                       |                        |
| $n_{im}$                                                    | 1.40                  |                        |                       |                        |
| $\kappa^2$                                                  | 2/3                   |                        |                       |                        |

[a] The depolarization time of all species are given together with their amplitudes in *Supplementary Table N1.2*.

[b] The fluorescence lifetimes of all species are given together with their species fractions in *Supplementary Table N1.1*.

[c] Measured relative to Rhodamine 6G in air-saturated Ethanol with  $\Phi_{F,Rh6G}=0.95$ . In the same measurement we obtained for the free dye  $\Phi_{F,Atto550} = 0.8 \pm 0.014$  and  $\tau_{Atto550} = 3.60 \text{ ns} \pm 2 \%$ , which corresponds to the values given by the manufacturer.

[d] The following reference values for the free dyes in solution were used from the manufacturers to scale the fluorescence quantum via the fluorescence lifetime of the free dye:

$\Phi_{F,Atto647N} = 0.65$ ;  $\Phi_{F,Alexa647} = 0.33$ ;  $\tau_{Atto647N} = 3.5 \text{ ns}$ ;  $\tau_{Alexa647} = 1.0 \text{ ns}$ .

A fluorescence lifetime analysis to relate the quantum yield  $\Phi'_F$  and lifetime  $\tau'$  specified by the manufacturer to the measured lifetime  $\tau$  and quantum yield  $\Phi_F$ :

$$\Phi_F = \Phi'_F \cdot \tau / \tau'$$

Here, we assume that the manufacturer  $\Phi'_F$  is correct, that the radiative constant is unchanged and that the lifetime decay is monoexponential. For many dyes in distinct environments, this might not be the case.

## Supplementary Note 1: Time-resolved experiments

### Global fit of the time-resolved polarized and magic angle fluorescence ensemble data

All polarization resolved fluorescence decay curves ( $F_{VV}(t), F_{VH}(t)$ ) with the Polarizer / Analyzer settings (Vertical,  $V$  /Horizontal,  $H$ ) of singly labeled molecules were studied in ensemble experiments in the Seidel lab by high-precision time correlated single-photon counting and were fitted jointly with corresponding magic angle ( $M$ ) fluorescence decay  $f_{VM}(t) = (f(t))$ . To reduce the number of parameters in the fits we used the so called homogenous approximation<sup>3</sup>. We assumed that de-excitation and depolarization of dyes are independent, i.e. in each donor de-excitation state dyes are characterized by the same set of depolarization times. For this case we can write model functions for the decay of the excited state population  $f(t)$  and the fluorescence anisotropy  $r(t)$ :

$$f_{VV}(t) = f(t)[1 + 2r(t)] \quad (1.1)$$

$$f_{VH}(t) = f(t)[1 - r(t)] \quad (1.2)$$

$$\text{with } f(t) = \sum_i x_i e^{-t/\tau_i} \quad \text{and } r(t) = \sum_j b^{(j)} e^{-t/\rho_j}$$

Here,  $\tau$  is the fluorescence lifetime and  $\rho$  is the depolarization times.  $x_i$  is (with  $\sum_i x^{(i)} = 1$ ) the species fraction of molecules having the lifetime  $\tau_i$  and the factor  $b_j$  is fraction of molecules having the depolarization time  $\rho_j$  where the fundamental anisotropy  $r_0$  is given by  $\sum_j b^{(j)} = r_0$  and the residual anisotropy is given by  $b^{(3)} = r_\infty$ . A maximum of three species for  $i$  and  $j$  were necessary to obtain satisfactory fits judged by  $\chi^2_r$ .

To fit real experimental decays IRF, background and amplitudes of the  $VV$ ,  $VH$  signals are accounted as:

$$F_{VV}(t) = F_0 \cdot IRF_{VV}(t) \otimes f_{VV}(t) + B_{VV} \quad (1.3)$$

$$F_{VH}(t) = g_{VV/VH} F_0 \cdot IRF_{VH}(t) \otimes f_{VH}(t) + B_{VH} \quad (1.4)$$

Where  $g_{VV/VH}$  is a correction factor for a polarization dependent detection efficiency,  $F_0$  - amplitude scaling factor,  $IRF_{VV}(t)$ ,  $IRF_{VH}(t)$  - instrument response functions and  $B_{VV}$ ,  $B_{VH}$  - background values. The “ $\otimes$ ” sign designates circular convolution.

The fit results for fluorescent signal in parallel and perpendicular polarization planes with respect to the vertically polarized excitation light with their rotation correlation times and amplitudes for D-only and A-only labeled DNA are presented in *Supplementary Tables N1.1 and N1.2*. The measured data and fitted curves with their weighted residuals are presented in the first column of the *Supplementary Figure N1*. Typical magic angle fluorescence decays are shown in the right column of the *Supplementary Figure N1*.

As expected<sup>4</sup>, the amplitude  $b_l$  for the fast depolarization motion with  $\rho_l$  is approximately a factor 2 larger for dyes where the transition dipole moment is more perpendicular to the linker (disc case: Alexa 488 and Alexa594) than for dyes with a more parallel the transition dipole moment (cone case: Atto550, Atto647N and Alexa647) (compare *Supplementary Figure 1* and *Supplementary Table N1.2*). Note that some dyes (e.g. Alexa488 and Alexa594) depolarize especially fast, because they have a large fraction of the fastest depolarization time such that  $k_{rot} \gg k_{FRET}$  might be satisfied for even higher FRET efficiencies. The depolarization of these dyes is best described by a disc model<sup>2</sup>.

**Supplementary Table N1.1:** Fluorescence lifetimes  $\tau_i$  and their amplitudes  $x_i$  for all studied Donor-only (DO) and Acceptor-only samples (AO). The quality of the fits was judged by  $\chi^2_r$ . [a,b]

| Base position (Linker), strand | Dye [c]  | Sample (DO or AO)    | $\tau_1$ [ns] ( $x_1$ ) | $\tau_2$ [ns] ( $x_2$ ) | $\tau_3$ [ns] ( $x_3$ ) | $\langle \tau \rangle_x$ [ns] | $\chi^2_r$ |
|--------------------------------|----------|----------------------|-------------------------|-------------------------|-------------------------|-------------------------------|------------|
| T 31(C2), D-strand             | Atto550  | 1-lo (DO), 2-lo (DO) | 0.74 (0.03)             | 3.47 (0.59)             | 4.44 (0.38)             | 3.76                          | 1.03       |
| T 23(C2), D-strand             | Atto550  | 1-hi (DO), 2-hi (DO) | 0.86 (0.03)             | 3.54 (0.63)             | 4.59 (0.34)             | 3.81                          | 1.02       |
| T 31(C2), A-strand             | Atto647N | 1-(AO), 3-(AO)       | 0.24 (0.04)             | 3.40 (0.52)             | 4.19 (0.44)             | 3.62                          | 1.03       |
| T 31 (C2), A-strand            | Alexa647 | 2 -(AO)              | 0.66 (0.05)             | 1.18 (0.90)             | 1.90 (0.05)             | 1.19                          | 1.00       |
| T 31(C6), D-strand             | Alexa488 | 3-lo (DO)            | 0.36 (0.03)             | 2.37 (0.05)             | 4.11 (0.92)             | 3.91                          | 1.03       |
| T 23(C6), D-strand             | Alexa488 | 3-hi (DO)            | 0.37 (0.04)             | 2.70 (0.04)             | 4.13 (0.92)             | 3.92                          | 1.08       |
| T 31 (C6), A-strand            | Alexa594 | 4-(AO)               | 0.31 (0.03)             | 3.76 (0.64)             | 4.55 (0.33)             | 3.91                          | 0.99       |

[a] in 20mM MgCl<sub>2</sub>, 5mM NaCl, 5mM TRIS at pH 7.5 measurement buffer.

[b] typical errors: average lifetime:  $\tau$ :  $\pm 0.02$  ns. Three lifetime: shortest lifetime  $\tau_1 \pm 20\%$  (with  $x_1 \sim 15\%$ ),  $\tau_2 \pm 10\%$  (with  $x_2 \sim 25\%$ ),  $\tau_3 \pm 3\%$  (with  $x_3 \sim 15\%$ ).

[c] Spectral settings:

**Atto550** (fluor. max 574 nm): excitation wavelength 552 nm, emission wavelength 580 nm (bandpass 5.4 nm).

**Atto647N** (fluor. max 664 nm): excitation wavelength 635 nm, emission wavelength 665 nm (bandpass 9.2 nm).

**Alexa647** (fluor. max 665 nm): excitation wavelength 635 nm, emission wavelength 665 nm (bandpass 8.1 nm).

**Alexa488** (fluor. max 525 nm): excitation wavelength 485 nm, emission wavelength 520 nm (bandpass 9.2 nm).

**Alexa594** (fluor. max 617 nm): excitation wavelength 590 nm, emission wavelength 617 nm (bandpass 8.1 nm).

Note that the fluorescence lifetime analysis exhibited signatures of solvent relaxation. Therefore we use wide bandpasses.

*Supplementary Table N1.2:* Rotation correlation times  $\rho_i$  with correspondent amplitudes  $b_i$  for Donor-only (DO) ( $r_0 = 0.38$ ) and Acceptor-only (AO) ( $r_0 = 0.38$ ) samples. The  $1\sigma$  confidence range for the longest correlation time is indicated in square brackets. The fit model is described by eqs 1.1-1.2 with the model functions eqs. 1.3-1.4. The quality of the fits was judged by  $\chi^2_r$ .

| Base position<br>(Linker),strand | dye          | Sample<br>(DO or<br>AO) | $\rho_1$ [ns]<br>( $b_1$ ) | $\rho_2$ [ns]<br>( $b_2$ ) | $\rho_3$ [ns] (1 $\sigma$ conf.)<br>( $b_3 = r_\infty$ ) [b] | $\chi^2_r$ |
|----------------------------------|--------------|-------------------------|----------------------------|----------------------------|--------------------------------------------------------------|------------|
| T 31(C2), D-strand               | Atto550      | 1-lo (DO),<br>2-lo (DO) | 0.63<br>(0.14)             | 3.08<br>(0.16)             | 174 [97-540]<br>(0.08)                                       | 1.04       |
| T 23(C2), D-strand               | Atto550      | 1-hi (DO),<br>2-hi (DO) | 0.58<br>(0.12)             | 2.76<br>(0.15)             | 63 [50-86]<br>(0.11)                                         | 1.01       |
| T 31(C2), A-strand               | Atto647N     | 1-(AO),<br>3-(AO)       | 0.41<br>(0.14)             | 2.05<br>(0.17)             | 46 [37-62]<br>(0.07)                                         | 1.01       |
| T 31 (C2), A-strand              | Alexa647 [a] | 2 -(AO)                 | 0.32<br>(0.09)             | 1.14<br>(0.23)             | 1e5 [125- $\infty$ ]<br>(0.06)                               | 0.99       |
| T 31(C6), D-strand               | Alexa488     | 3-lo (DO)               | 0.25<br>(0.22)             | 1.31<br>(0.12)             | 31 [24-42]<br>(0.04)                                         | 1.03       |
| T 23(C6), D-strand               | Alexa488     | 3-hi (DO)               | 0.26<br>(0.22)             | 1.43<br>(0.12)             | 37 [31-46]<br>(0.04)                                         | 1.04       |
| T 31 (C6), D-strand              | Alexa594     | 4-(AO)                  | 0.46<br>(0.22)             | 1.88<br>(0.09)             | 77 [58-121]<br>(0.07)                                        | 1.02       |

[a] Only VV, VH depolarization curves used for fitting in this case.

[b] Due to fluctuations in the G-factor determinations we have small systematic errors; i.e.  $\rho_3 > 20$  ns and not the fitted value

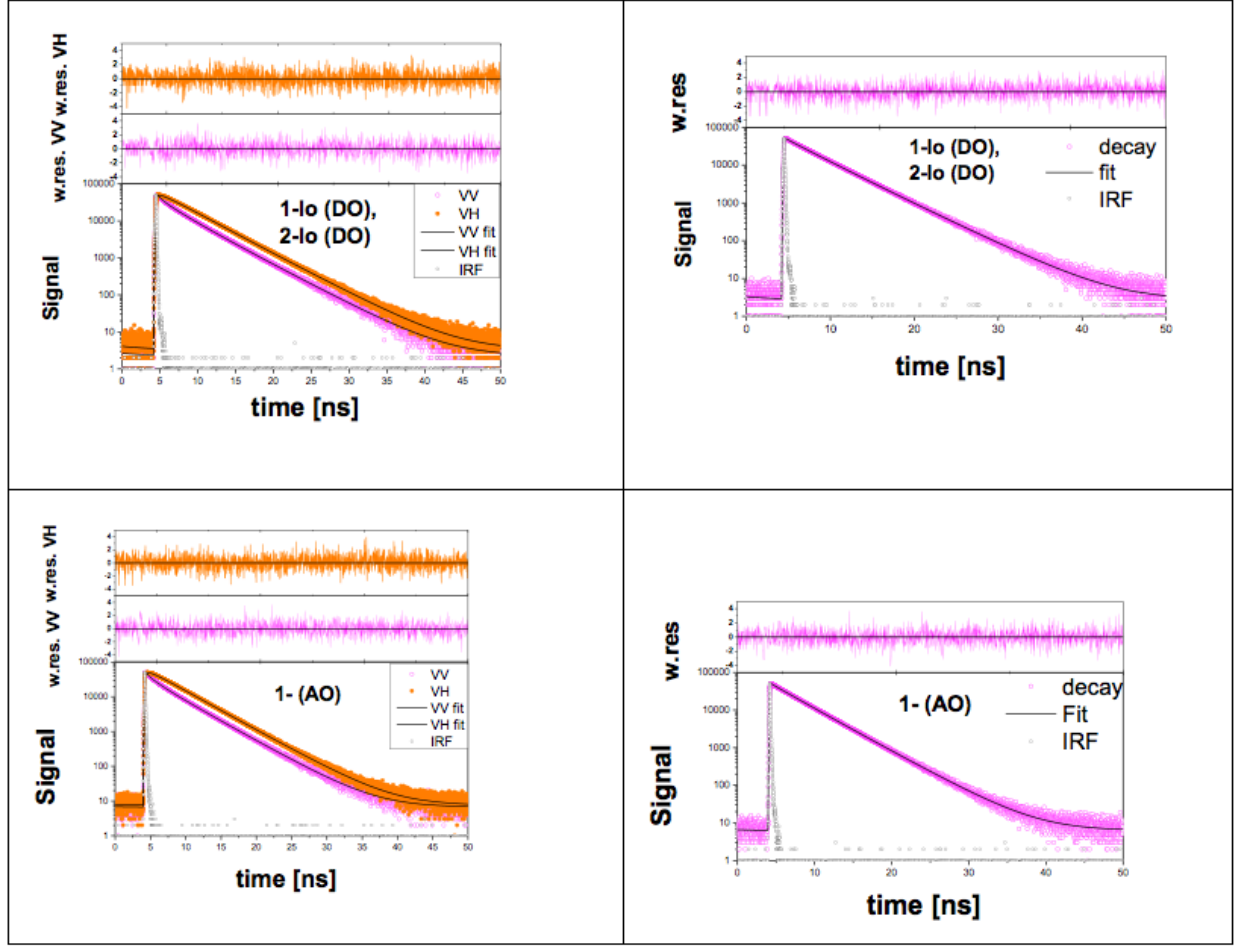

**Supplementary Figure N1:** Left pannels: Typical fluorescent signal in parallel and perpendicular polarization channels (magenta and orange) with the corresponding fits (black) for 1-lo (DO), 2-lo (DO), 1-(AO) samples with weighted residuals on the top. Right pannels: the corresponding magic angle fluorescence decay curves with weighted residuals on the top. The fit results are displayed in *Supplementary Tables N1.1 and N1.2* using fit procedure described by eqs 1.1-1.2 with the model functions eqs 1.3-1.4. The quality of the fits was judged by  $\chi^2_r$ .

### **Species average lifetime determination**

Magic angle fluorescence decays were described with three fluorescence lifetimes  $\tau_i$  and the species fractions  $x_i$  and thus species averaged lifetime  $\langle\tau\rangle_x$  was calculated as:

$$\langle\tau\rangle_x = x_1\tau_1 + x_2\tau_2 + x_3\tau_3 \quad (1.5)$$

### **Experimental deviations obtained during lifetime-based experiments**

The lifetime-based measurements had a significantly lower precision and accuracy than intensity-based measurements. The following factors might be responsible for the observed deviations in the fluorescence lifetime-based FRET experiments:

1. The precision propagates differently for intensity based and time-resolved techniques. In intensity-based FRET measurements the relative error of a normalized donor-acceptor distance changes less with increasing distance. The precision of time-resolved FRET



measurements is highest for small DA distances (the minimum is  $R_{DA}/R_0 \approx 0.7$ ) which were not the focus of this study <sup>1</sup>.

2. Time-resolved techniques strongly depend on a representative (chemically equivalent) Donor-only reference sample that is crucial for resolving large distances accurately.
3. If in the ensemble measurements the FRET sample contains also molecules which are labeled with a donor, it becomes very difficult to resolve species with low FRET efficiencies.
4. The accuracy of time-resolved FRET measurements depends on an appropriate fit model. It is crucial to consider the heterogeneity of the donor lifetimes and dye-linker distributions (eq. 27 in ref. <sup>3</sup>). Moreover the analysis model should allow fitting a variable fraction of donor-only species, which was needed for all provided samples. Altogether, this results in complex fit models which are not widely used in the FRET community because they are difficult to implement in commercial software. In contrast, some groups analyzed the donor decays by a simple series of exponentials, which results in a systematic shift of the obtained FRET parameters.

Thus all four effects in time-resolved FRET measurements contributed to the fact that the precision and accuracy of the distances recovered especially for all lo-samples was markedly lower than that of intensity-based methods.

## Supplementary Note 2: AV simulations to compute donor acceptor distances

The model for the double-stranded B-DNA is generated using the Nucleic Acid Builder version 04/17/2017 for Amber<sup>5</sup> (see Figure 1, main text). For modelling the dye molecule, we use a geometrical approach that considers sterically allowed dye positions within the linker length from the attachment point with equal probability. This defines the accessible volume (AV)<sup>6</sup>. The dye molecules are modeled as ellipsoids (approximated by three radii; AV3-Model) and AVs are generated using the FPS software<sup>7</sup>. For the distance computation a dye pair specific Förster Radius is used; i.e., it is assumed that within the AV the dye molecule samples all positions isotropically, however, for a single excitation it is at a fixed position. Moreover, it is assumed that dye rotation is so fast, that all possible orientations are sampled during the fluorescence lifetime and thus the factor  $\langle \kappa^2 \rangle = 2/3$  (isotropic coupling).

The boundary tolerance (called ‘allowed sphere’ in the FPS software) is used to ignore small residues that are fixed in the PDB-model, but flexible in solution. The larger this value, the larger the structural parts that are ignored for the AV generation. The labelling position is the C7 of the thymine (the C-atom of the thymine’s methyl group). All mean geometric dyes parameters are estimated with ChemDraw software (see *Supplementary Table N2.1*). Further used parameters are: Boundary tolerance 0.5, accessible volume grid (rel.) 0.2; Min. grid [Å] 0.4, Search nodes: 3 and E samples: 200.

*Supplementary Table N2.1*: Recommended dye parameters for the AV simulations with AV3-model.

|                | linker length<br>[Å] | linker width<br>[Å] | R1<br>[Å] | R2<br>[Å] | R3<br>[Å] |
|----------------|----------------------|---------------------|-----------|-----------|-----------|
| dT-C6-Alexa488 | 20.5                 | 4.5                 | 5.0       | 4.5       | 1.5       |
| dT-C2-Atto550  | 20.4                 | 4.5                 | 7.1       | 5.0       | 1.5       |
| dT-C6-Alexa594 | 20.0                 | 4.5                 | 8.1       | 3.2       | 2.6       |
| dT-C2-Alexa647 | 21.0                 | 4.5                 | 11.0      | 4.7       | 1.5       |
| dt-C2-Atto647N | 20.4                 | 4.5                 | 7.2       | 4.5       | 1.5       |

**Error estimation.** For each sample the distances between mean dye positions ( $R_{MP}^{model}$ ) and expected experimentally observed apparent distance  $R_{(E)}^{model}$  are calculated (see *Table 4*, main text). The error for the model distances is estimated by varying the linker lengths (from 10 to 21 Å), linker width (from 4.0 to 5.0 Å), the dye model (single sphere with the radius 6 Å (AV1 model) and ellipsoid with three radii R1=7.1 Å, R2=4.5 Å and R3=1.8 Å (AV3 model) and the boundary tolerance between dye and DNA (0.5 and 1.5 Å). The standard deviation of all DA distances computed by FPS was used as error.

### Supplementary Note 3: $R_{E\}$ to $R_{MP}$ conversion

For the conversion between  $R_{E\}$  and  $R_{MP}$  we distinguish two cases, a known and unknown environment of the dye molecule:

**Case 1**, the local environment of the dye molecule is known. Here, we use average (apparent) distances from different data-sources, i.e.,  $R_{E\}$  from experiment, and  $R_{MP}$  from coarse-grained-structural modeling to generate conversion functions. Typically, we use coarse-grained simulations to approximate accessible volumes (AVs) for biomolecules<sup>7</sup>. These AVs are translated / rotated and the average apparent DA distance ( $R_{E\}$ ) and the distance  $R_{MP}$  are calculated, which introduces noise. The resulting conversion tables are approximated by third order polynomials. Here we used the AVs for the samples 1,2,3,4 low and high FRET correspondingly. For the polynomial  $R_{MP} = (a_0 + a_1 R_{E\} + a_2 R_{E\}^2 + a_3 R_{E\}^3)$  the coefficients are given in the *Supplementary Table N3.1* for all FRET pairs.

Note that the conversion functions are specific for the chosen dye pair because they depend on the Förster Radius of the FRET pair and the used dye parameters for the AV simulation. The differences between AVs in different molecular environments (DNA or protein) become smaller the less restricted the dye is. The offset of the conversion function depends on the size of the dye spheres and the linker lengths.

**Supplementary Table N3.1.** Conversion polynomial for  $R_{MP} = (a_0 + a_1 R_{E\} + a_2 R_{E\}^2 + a_3 R_{E\}^3)$  using the dye pair specific  $R_0$  and specific AVs of the samples 1, 2, 3 and 4, respectively. Note that these polynomials are only valid for this specific geometry and dyes.

| FRET pair         | $R_0$ [Å] | $a_0$ [Å] | $a_1$ | $a_2$ [Å] <sup>-1</sup> | $a_3$ [Å] <sup>-2</sup> |
|-------------------|-----------|-----------|-------|-------------------------|-------------------------|
| Atto550-Atto647N  | 62.6      | -41.8     | 2.13  | $-0.92 \cdot 10^{-2}$   | $2.40 \cdot 10^{-5}$    |
| Atto550-Alexa647  | 68.0      | -40.3     | 1.99  | $-0.74 \cdot 10^{-2}$   | $1.67 \cdot 10^{-5}$    |
| Alexa488-Atto647N | 49.3      | -53.8     | 2.83  | $-1.89 \cdot 10^{-2}$   | $6.17 \cdot 10^{-5}$    |
| Alexa488-Alexa594 | 57.0      | -43.9     | 2.24  | $-1.02 \cdot 10^{-2}$   | $2.48 \cdot 10^{-5}$    |

**Case 2**, the local environment of the dye molecule is not known. Here, we make the most general assumption that the AV can be approximated by a sphere with its radius estimated from the size of the dye and linker length (slightly smaller than the dye and linker length). This allows us to estimate the conversion of  $R_{E\}$  to  $R_{MP}$  by performing Monte Carlo simulations<sup>8</sup>. In the Monte Carlo simulation, we place 10,000 positions uniformly distributed within a sphere of 18 Å radius for both dyes. For a given distance of the mean position of these spheres ( $R_{MP}$ ) we calculate the respective FRET efficiencies via the Förster formula with an orientation factor of  $\kappa^2 = 2/3$ . The mean of these values is an unbiased estimate for the expected value of the FRET efficiency. We vary the mean position distance from 0.5  $R_0$  to 1.5  $R_0$  and fit the resulting means with a third order polynomial (coefficients  $a_0$ ,  $a_1$ ,  $a_2$  and  $a_3$ ). For convenience the conversion coefficients for a large range of used Förster radii were determined and given here in *Supplementary Table N3.2*. The equivalence of both approaches is demonstrated in *Supplementary Figure N3.1* for the dye pair Atto550-Atto647N.

**Supplementary Table N3.2.:** Coefficients for the conversion polynomials  $R_E$  to  $R_{MP}$  for case 2. These are valid for the specified Förster radius  $R_0$ .

| $R_0$ [Å] | $a_0$ [Å] | $a_1$ | $a_2$ [Å] <sup>-1</sup> | $a_3$ [Å] <sup>-2</sup> |
|-----------|-----------|-------|-------------------------|-------------------------|
| 50        | -33.6     | 1.65  | $3.25 \cdot 10^{-3}$    | $-7.26 \cdot 10^{-5}$   |
| 51        | -34.0     | 1.70  | $1.55 \cdot 10^{-3}$    | $-5.68 \cdot 10^{-5}$   |
| 52        | -33.0     | 1.64  | $2.25 \cdot 10^{-3}$    | $-5.85 \cdot 10^{-5}$   |
| 53        | -31.7     | 1.57  | $2.93 \cdot 10^{-3}$    | $-5.91 \cdot 10^{-5}$   |
| 54        | -32.8     | 1.64  | $1.27 \cdot 10^{-3}$    | $-4.65 \cdot 10^{-5}$   |
| 55        | -32.0     | 1.61  | $1.43 \cdot 10^{-3}$    | $-4.46 \cdot 10^{-5}$   |
| 56        | -30.0     | 1.51  | $2.78 \cdot 10^{-3}$    | $-4.98 \cdot 10^{-5}$   |
| 57        | -30.0     | 1.51  | $2.19 \cdot 10^{-3}$    | $-4.39 \cdot 10^{-5}$   |
| 58        | -30.0     | 1.52  | $1.73 \cdot 10^{-3}$    | $-3.91 \cdot 10^{-5}$   |
| 59        | -27.7     | 1.42  | $3.03 \cdot 10^{-3}$    | $-4.37 \cdot 10^{-5}$   |
| 60        | -29.1     | 1.49  | $1.55 \cdot 10^{-3}$    | $-3.42 \cdot 10^{-5}$   |
| 61        | -27.5     | 1.42  | $2.36 \cdot 10^{-3}$    | $-3.67 \cdot 10^{-5}$   |
| 62        | -26.5     | 1.37  | $2.77 \cdot 10^{-3}$    | $-3.74 \cdot 10^{-5}$   |
| 63        | -27.3     | 1.42  | $1.67 \cdot 10^{-3}$    | $-2.99 \cdot 10^{-5}$   |
| 64        | -25.6     | 1.35  | $2.56 \cdot 10^{-3}$    | $-3.28 \cdot 10^{-5}$   |
| 65        | -26.1     | 1.38  | $1.88 \cdot 10^{-3}$    | $-2.83 \cdot 10^{-5}$   |
| 66        | -26.4     | 1.39  | $1.42 \cdot 10^{-3}$    | $-2.50 \cdot 10^{-5}$   |
| 67        | -24.9     | 1.33  | $2.07 \cdot 10^{-3}$    | $-2.69 \cdot 10^{-5}$   |
| 68        | -24.1     | 1.30  | $2.27 \cdot 10^{-3}$    | $-2.68 \cdot 10^{-5}$   |
| 69        | -24.2     | 1.31  | $1.90 \cdot 10^{-3}$    | $-2.39 \cdot 10^{-5}$   |
| 70        | -23.3     | 1.28  | $2.29 \cdot 10^{-3}$    | $-2.49 \cdot 10^{-5}$   |
| 71        | -24.4     | 1.33  | $1.30 \cdot 10^{-3}$    | $-1.95 \cdot 10^{-5}$   |
| 72        | -23.4     | 1.29  | $1.80 \cdot 10^{-3}$    | $-2.11 \cdot 10^{-5}$   |
| 73        | -22.6     | 1.27  | $1.86 \cdot 10^{-3}$    | $-2.04 \cdot 10^{-5}$   |
| 74        | -23.0     | 1.28  | $1.53 \cdot 10^{-3}$    | $-1.84 \cdot 10^{-5}$   |
| 75        | -22.4     | 1.26  | $1.62 \cdot 10^{-3}$    | $-1.80 \cdot 10^{-5}$   |
| 76        | -21.8     | 1.24  | $1.70 \cdot 10^{-3}$    | $-1.77 \cdot 10^{-5}$   |
| 77        | -21.6     | 1.24  | $1.58 \cdot 10^{-3}$    | $-1.66 \cdot 10^{-5}$   |
| 78        | -21.8     | 1.25  | $1.28 \cdot 10^{-3}$    | $-1.47 \cdot 10^{-5}$   |
| 79        | -21.2     | 1.23  | $1.44 \cdot 10^{-3}$    | $-1.49 \cdot 10^{-5}$   |
| 80        | -21.2     | 1.24  | $1.32 \cdot 10^{-3}$    | $-1.41 \cdot 10^{-5}$   |
| 81        | -20.5     | 1.22  | $1.43 \cdot 10^{-3}$    | $-1.39 \cdot 10^{-5}$   |
| 82        | -20.3     | 1.21  | $1.40 \cdot 10^{-3}$    | $-1.34 \cdot 10^{-5}$   |
| 83        | -20.5     | 1.22  | $1.17 \cdot 10^{-3}$    | $-1.20 \cdot 10^{-5}$   |
| 84        | -19.8     | 1.20  | $1.36 \cdot 10^{-3}$    | $-1.24 \cdot 10^{-5}$   |
| 85        | -20.3     | 1.22  | $0.96 \cdot 10^{-3}$    | $-1.05 \cdot 10^{-5}$   |
| 86        | -19.5     | 1.19  | $1.20 \cdot 10^{-3}$    | $-1.10 \cdot 10^{-5}$   |
| 87        | -19.1     | 1.18  | $1.22 \cdot 10^{-3}$    | $-1.08 \cdot 10^{-5}$   |
| 88        | -19.0     | 1.18  | $1.15 \cdot 10^{-3}$    | $-1.02 \cdot 10^{-5}$   |
| 89        | -19.0     | 1.18  | $1.04 \cdot 10^{-3}$    | $-0.95 \cdot 10^{-5}$   |
| 90        | -18.8     | 1.18  | $0.99 \cdot 10^{-3}$    | $-0.91 \cdot 10^{-5}$   |

We tested that the polynomials derived using case 1 or case 2 generally yield almost identical conversion functions (*Supplementary Figure N3.1*).

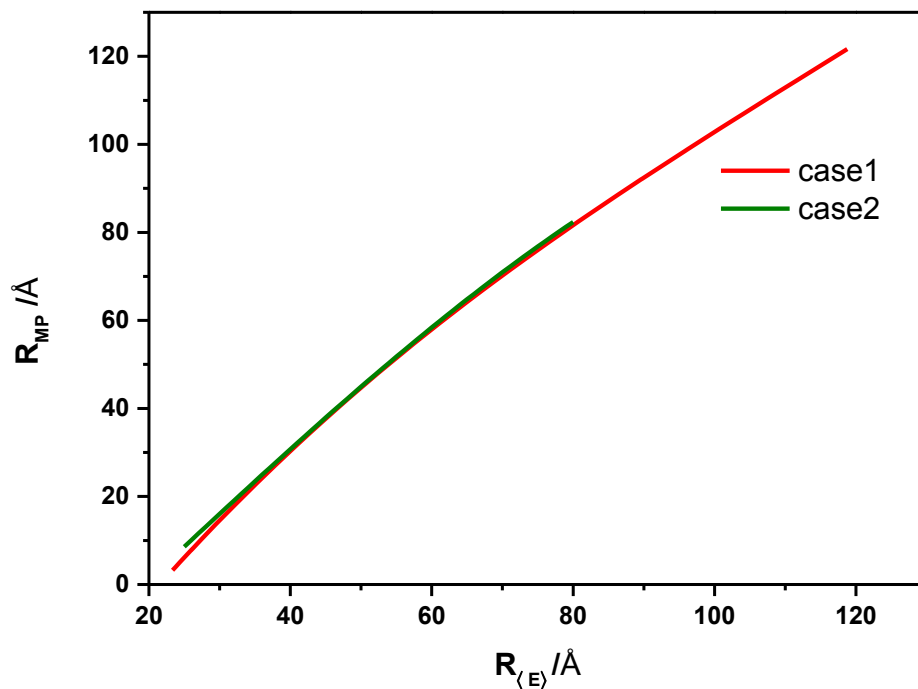

**Supplementary Figure N3.1.** Polynomial  $R_{MP} = a_0 + a_1 R_{(E)} + a_2 R_{(E)}^2 + a_3 R_{(E)}^3$  for the dye pair Atto550-Atto647N with AVs for DNA (case 1:  $R_0 = 62.6 \text{\AA}$ ) and with the approximation by a sphere (case 2:  $R_0 = 62.0 \text{\AA}$ ). Interpolated points in steps of  $1 \text{\AA}$ .

## Supplementary Note 4: Error propagation

Based on the measurements of sample 1-lo and 1-hi, we performed an error propagation using  $\Delta E = 0.033$  (which was the precision for these two best investigated samples). *Figure 5* follows from the following distance uncertainty:

$$\Delta R(R_0, \Delta R_0, \Delta E | R) = \sqrt{\left(\frac{\partial R(R_0, E)}{\partial R_0} \cdot \Delta R_0\right)^2 + \left(\frac{\partial R(R_0, E)}{\partial E} \cdot \Delta E\right)^2} = \sqrt{\left(\frac{R}{R_0} \cdot \Delta R_0\right)^2 + \left(\frac{1}{6} \left(1 + \left(\frac{R}{R_0}\right)^6\right)^2 \left(\frac{R}{R_0}\right)^{-5} R_0 \cdot \Delta E\right)^2} \quad (4.1)$$

In the following, we performed more detailed error propagation with disentangled error sources. We estimate the uncertainties of all quantities separately and propagate them towards an uncertainty in the distance. The overall uncertainty in the distance is given by:

$$\Delta R(R_0, \Delta R_0, \gamma, \Delta \gamma, \langle F \rangle, \Delta I_{Dem|Dex}^{(BG)}, \Delta I_{Aem|Dex}^{(BG)}, \Delta \beta, \Delta \alpha | R) = \sqrt{\Delta R_{R_0}^2 + \Delta R_{\gamma}^2 + \Delta R_{bgD}^2 + \Delta R_{bgA}^2 + \Delta R_{\alpha}^2 + \Delta R_{\delta}^2} \quad (4.2)$$

with the following error contribution for the Förster radius:

$$\Delta R_{R_0}(R) = R \frac{\Delta R_0}{R_0} \quad (4.3)$$

And the following error contribution for the gamma factor:

$$\Delta R_{\gamma}(R) = \frac{R}{6} \cdot \frac{\Delta \gamma}{\gamma} \quad (4.4)$$

And the following error contribution for the background in the donor channel after donor excitation:

$$\Delta R_{bgD}(R) = \frac{R}{6} \left[ \gamma \left(1 + \left(\frac{R_0}{R}\right)^6\right) + \alpha \left(1 + \left(\frac{R}{R_0}\right)^6\right) \right] \cdot \frac{\Delta I_{Dem|Dex}^{(BG)}}{\langle F \rangle} \quad (4.5)$$

And the following error contribution for the background in the acceptor channel after donor:

$$\Delta R_{bgA}(r) = -\frac{R}{6} \left(1 + \left(\frac{R}{R_0}\right)^6\right) \cdot \frac{\Delta I_{Aem|Dex}^{(BG)}}{\langle F \rangle} \quad (4.6)$$

And the following error contribution for the direct excitation factor of the acceptor with the green laser:

$$\Delta R_{\delta}(R) = -\frac{R}{6} \beta \left(1 + \left(\frac{R}{R_0}\right)^6\right) \cdot \Delta \delta \quad (4.7)$$

And the following error contribution for the leakage factor of donor fluorescence in the acceptor channel:

$$\Delta R_{\alpha}(R) = -\frac{R}{6} \frac{1}{\gamma} \left(\frac{R}{R_0}\right)^6 \cdot \Delta \alpha \quad (4.8)$$

Please note that for determination of background we set  $\gamma = \beta = 1$  and  $\alpha = \delta = 0$ . This represents the ideal values. Further parameters and uncertainties are taken from the reference lab:  $\Delta \gamma / \gamma = 0.1$ ,  $\langle F \rangle = 50$ ,  $\Delta I_{Dem|Dex}^{(BG)} = 1$ ,  $\Delta I_{Aem|Dex}^{(BG)} = 1$ ,  $\Delta \delta / \delta = 0.1$ ,  $\Delta \alpha / \alpha = 0.1$ ,  $\Delta R_0 = 0.07$ . See *Online Methods, Section 2 and 3* for the nomenclature and details on the Förster radius.  $\langle F \rangle$  is the average sum of the corrected donor and acceptor fluorescence.

The above error analysis is based on  $R_{DA}$  and may be further propagated to the apparent donor-acceptor distance  $R_{\langle E \rangle}$  and the distance between the mean positions of the dyes,  $R_{MP}$ , when the above model assumption of a freely rotating and diffusing dye is applied. This becomes very involved and does not show significant deviations from *Figure 5* in the main text.

## Supplementary Note 5: Further samples

| Name         | Base position (Linker), strand           | Dyes (Donor/ Acceptor)                                                      | Sequence                                                                                                                                                   |
|--------------|------------------------------------------|-----------------------------------------------------------------------------|------------------------------------------------------------------------------------------------------------------------------------------------------------|
| <b>3-lo</b>  | T 31(C6), D-strand<br>T 31(C2), A-strand | Alexa488<br>Tetrafluorophenyl Ester/<br>Atto647N NHS                        | 5' - GAG CTG AAA GTG TCG AGT TTG TTT GAG TGT <b>TTG</b> TCT GG-3'<br>3' - CTC GAC <b>T</b> <b>TT</b> CAC AGC TCA AAC AAA CTC ACA AAC AGA CC-5'<br>- biotin |
| <b>3-hi:</b> | T 23(C6), D-strand<br>T 31(C2), A-strand | Alexa488<br>Tetrafluorophenyl Ester/<br>Atto647N NHS                        | 5' - GAG CTG AAA GTG TCG AGT TTG <b>TTT</b> GAG TGT TTG TCT GG-3'<br>3' - CTC GAC <b>T</b> <b>TT</b> CAC AGC TCA AAC AAA CTC ACA AAC AGA CC-5'<br>-biotin  |
| <b>4-lo:</b> | T 31(C6), D-strand<br>T 31(C6), A-strand | Alexa488<br>Tetrafluorophenyl Ester/<br>Alexa594<br>Tetrafluorophenyl Ester | 5' - GAG CTG AAA GTG TCG AGT TTG TTT GAG TGT <b>TTG</b> TCT GG-3'<br>3' - CTC GAC <b>T</b> <b>TT</b> CAC AGC TCA AAC AAA CTC ACA AAC AGA CC-5'<br>- biotin |
| <b>4-hi:</b> | T 23(C6), D-strand<br>T 31(C6), A-strand | Alexa488<br>Tetrafluorophenyl Ester/<br>Alexa594<br>Tetrafluorophenyl Ester | 5' - GAG CTG AAA GTG TCG AGT TTG <b>TTT</b> GAG TGT TTG TCT GG-3'<br>3' - CTC GAC <b>T</b> <b>TT</b> CAC AGC TCA AAC AAA CTC ACA AAC AGA CC-5'<br>- biotin |

Even for samples 3 and 4 the precision of the hi-samples, where all individual FRET efficiencies were in a sensitive range of the specific dye pairs, is very good (2 - 4 %). Moreover, the experimental and model values of the low- and hi-samples agree very well with each other (the deviations range between 2 and 10 %). This suggests that we do not have dye artifacts for all four FRET pairs. The results obtained for the different FRET pairs will be important in the future to judge key aspects of different fluorophore properties.

## Supplementary Note 6: MD simulations

While the analysis in this paper used a static model for the double-stranded DNA structure, DNA is known to not be completely rigid<sup>9</sup>. Therefore, we performed Molecular dynamics (MD) simulations of the DNA molecule to explore its rigidity using the latest force fields which were reported to be consistent with experimental observables of the conformational flexibility of dsDNA.

The all-atom MD simulations were performed with the Amber16 suite of programs<sup>10</sup> using the bsc1 force field<sup>5</sup>. The initial structure of the B-DNA molecule, which was generated by 3D-DART (see main text), was placed in an octahedral box of TIP3P water molecules<sup>11</sup>, such that the distance between the edge of the water box and the closest DNA atom was at least 11 Å. MgCl<sub>2</sub> and NaCl were added to achieve concentrations of 20 mM and 10 mM, respectively. For Na<sup>+</sup> and Cl<sup>-</sup>, the parameters by Joung and Cheatham<sup>12</sup> were used, while for Mg<sup>2+</sup> the parameters by Li et al.<sup>13</sup> were used.

Each system was then prepared based on a protocol used earlier<sup>14</sup>. The simulation system was minimized by 200 steps of steepest descent and subsequently 50 steps of conjugate gradient minimization. The minimized system was heated from 100 to 300 K over 50 ps, and subsequently the solvent density was adjusted for 150 ps by NPT-MD simulation. During the previous two steps, harmonic force restraints were applied on all solute atoms with force constants of 5 kcal mol<sup>-1</sup> Å<sup>-2</sup>. These harmonic force restraints were gradually reduced to 1 kcal mol<sup>-1</sup> Å<sup>-2</sup> during 250 ps of NVT-MD simulation. This step was followed by 50 ps of NVT-MD simulation without positional restraints.

The time step for all MD simulations was 2 fs. Subsequently, we performed five independent MD simulations of 250 ns length each. Coordinates were extracted from the simulations every 20 ps. We used the FPS program<sup>7</sup> to calculate FRET efficiencies for the structural ensemble of the MD simulation, i.e. for each structure the AVs with the spatial dye (D and A) distributions is calculated and the average FRET efficiency is computed.

The ensembles from the MD simulations suggest that the DNA is not completely rigid, but exhibits some bending motion (*Supplementary Figure N.6.1*). The obtained distributions of FRET efficiencies show that the ensembles from the MD simulations yield comparable, but slightly lower mean FRET efficiencies and thus longer distances than for the static model (*Supplementary Figure N.6.2, Supplementary Table N.6.1*).



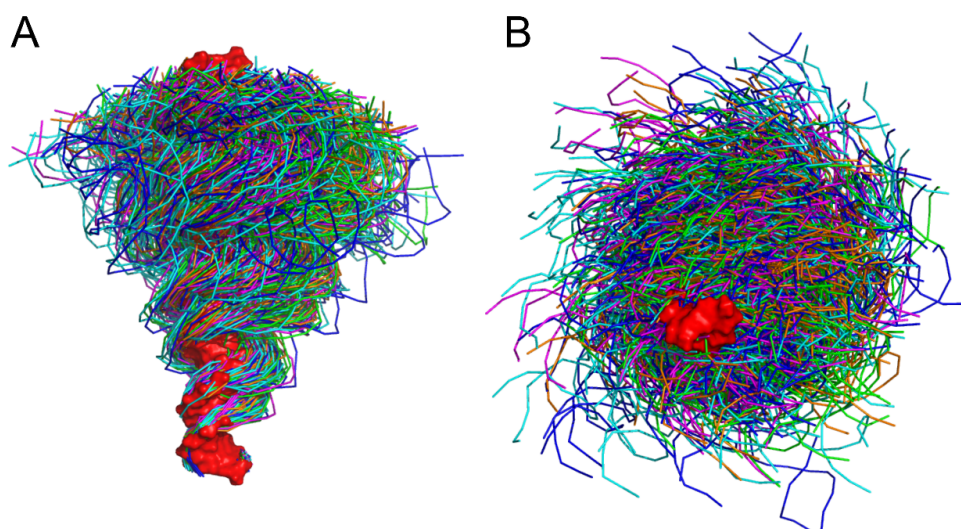

**Supplementary Figure N.6.1:** Structural ensembles from the MD simulations. The starting structure (red surface representation) was overlaid with conformations extracted from the MD simulations using the first 5 base pairs of the DNA. The five independent MD simulations are shown as differently colored ribbons (green, blue, orange, magenta, and cyan). For visibility, snapshots extracted every 2 ns were used for this representation. A: Side view; B: Top view.

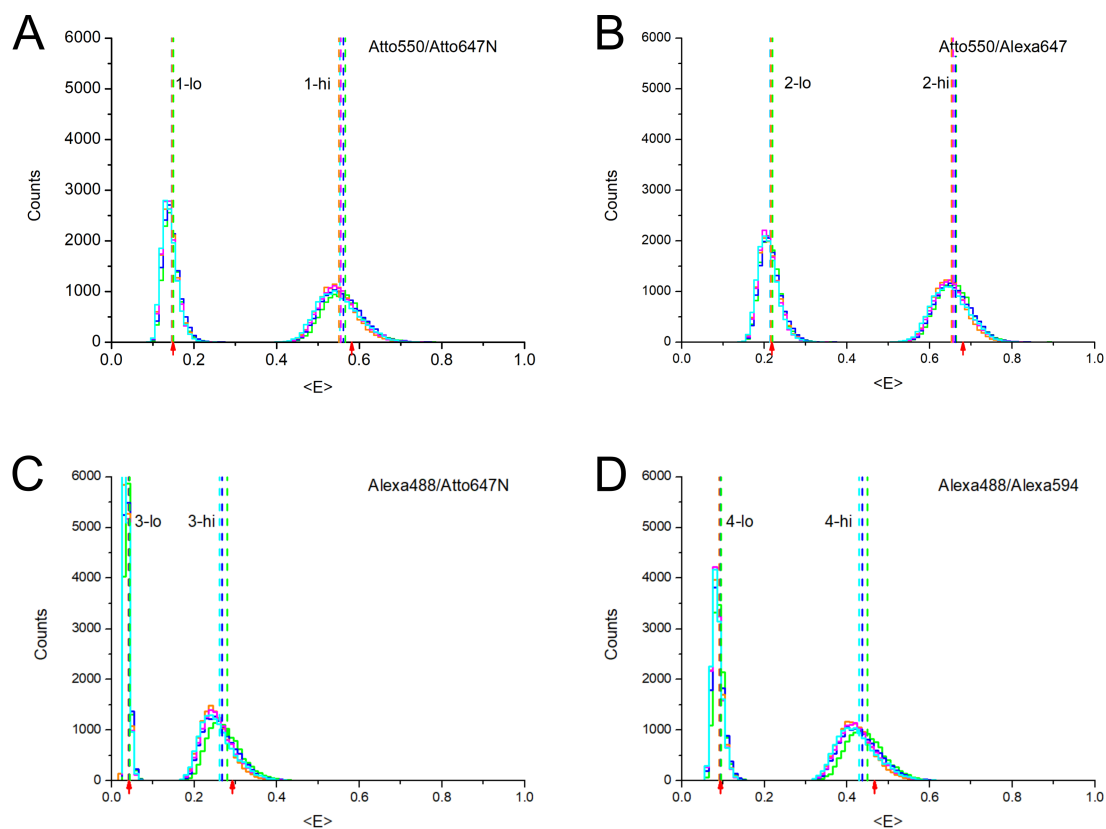

**Supplementary Figure N.6.2:** Distribution of FRET efficiencies calculated for the conformation extracted from the MD simulations for the four samples (A: Atto550/Atto647N, B: Atto550/Alexa647, C: Alexa488/Atto647N, D: Alexa488/Alexa594). The five colors (green, blue, orange, magenta, and cyan) correspond to the five independent MD simulations performed. Vertical dashed lines indicate the mean of the distribution, while the red arrows below the X-axis indicate the values calculated for the starting structure.

**Supplementary Table N.6.1:** Comparison of FRET efficiencies  $\langle E \rangle_{dyn}$  and corresponding DA distances  $R_{(E)}^{(dyn)}$  calculated from the five MD simulations to the values from experiments ( $\langle E \rangle_{exp}$ ,  $R_{(E)}^{(exp)}$ ) and the static model with  $\langle E \rangle_{static}$ .

| Sample                   | $\langle E \rangle_{dyn}$ <sup>[a]</sup> | $\langle E \rangle_{static}$ <sup>[b]</sup> | $\langle E \rangle_{exp}$ <sup>[c]</sup> | $R_{(E)}^{(dyn)}$ [Å] <sup>[d]</sup> | $R_{(E)}^{(exp)}$ [Å] <sup>[e]</sup> |
|--------------------------|------------------------------------------|---------------------------------------------|------------------------------------------|--------------------------------------|--------------------------------------|
| <b>Atto550/Atto647N</b>  |                                          |                                             |                                          |                                      |                                      |
| 1-lo                     | 0.15                                     | 0.15                                        | $0.15 \pm 0.02$                          | 83.9                                 | $83.4 \pm 2.5$                       |
| 1-hi                     | 0.56                                     | 0.58                                        | $0.56 \pm 0.03$                          | 60.3                                 | $60.3 \pm 1.3$                       |
| <b>Atto550/Alexa647</b>  |                                          |                                             |                                          |                                      |                                      |
| 2-lo                     | 0.22                                     | 0.22                                        | $0.21 \pm 0.04$                          | 84.2                                 | $85.4 \pm 3.4$                       |
| 2-hi                     | 0.66                                     | 0.68                                        | $0.60 \pm 0.05$                          | 61.0                                 | $63.7 \pm 2.3$                       |
| <b>Alexa488/Atto647N</b> |                                          |                                             |                                          |                                      |                                      |
| 3-lo                     | 0.04                                     | 0.04                                        | $0.04 \pm 0.02$                          | 83.1                                 | $89.5 \pm 12.3$                      |
| 3-hi                     | 0.27                                     | 0.29                                        | $0.24 \pm 0.04$                          | 58.4                                 | $60.1 \pm 2.3$                       |
| <b>Alexa488/Alexa594</b> |                                          |                                             |                                          |                                      |                                      |
| 4-lo                     | 0.09                                     | 0.09                                        | $0.13 \pm 0.06$                          | 83.5                                 | $79.6 \pm 6.2$                       |
| 4-hi                     | 0.44                                     | 0.47                                        | $0.41 \pm 0.04$                          | 59.5                                 | $60.7 \pm 1.7$                       |

[a] Calculated as average over the five simulations (the standard deviation is in all cases below 0.008).

[b] Calculated for the static starting structure.

[c] From measurements (cf. main text, *Table 4*).

[d] Calculated from  $\langle E \rangle_{dyn}$  using Formula (V) from *Table 1* in the main text.

[e] Calculated from experiments (cf. main text; *Table 4*).

## **Bibliography:**

1. Wozniak, A. K., Schröder, G. F., Grubmüller, H., Seidel, C. A. M. & Oesterhelt, F. Single-Molecule FRET Measures Bends and Kinks in DNA. *Proc. Natl. Acad. Sci. USA* **105**, 18337-18342 (2008).
2. Hellenkamp, B., Wortmann, P., Kandzia, F., Zacharias, M. & Hugel, T. Multidomain Structure and Correlated Dynamics Determined by Self-Consistent FRET Networks. *Nat. Meth.* **14**, 174-180 (2017).
3. Peulen, T. O., Opanasyuk, O. & Seidel, C. A. M. Combining graphical and analytical methods with molecular simulations to analyze time-resolved FRET-measurements of labeled macromolecules accurately. *J. Phys. Chem. B* **121**, 8211-8241 (2017).
4. Sindbert, S. *et al.* Accurate Distance Determination of Nucleic Acids via Förster Resonance Energy Transfer: Implications of Dye Linker Length and Rigidity. *J. Am. Chem. Soc.* **133**, 2463-2480 (2011).
5. Ivani, I. *et al.* Parmbsc1: a refined force field for DNA simulations. *Nat. Meth.* **13**, 55-58 (2016).
6. Muschielok, A. *et al.* A Nano-Positioning System for Macromolecular Structural Analysis. *Nat. Meth.* **5**, 965-971 (2008).
7. Kalinin, S. *et al.* A toolkit and benchmark study for FRET-restrained high-precision structural modeling. *Nat. Meth.* **9**, 1218-1227 (2012).
8. Eilert, T., Beckers, M., Drechsler, F. & Michaelis, J. Fast-NPS - A Markov chain Monte Carlo-based analysis tool to obtain structural information from single-molecule FRET measurements. *Comput. Phys. Commun.* **219**, 377-389 (2017).
9. Stelzl, L. S., Erlenbach, N., Heinz, M., Prisner, T. F. & Hummer, G. Resolving the conformational dynamics of DNA with Ångström resolution by pulsed electron-electron double resonance and molecular dynamics. *J. Am. Chem. Soc.* **139**, 11674-11677 (2017).
10. Case, D. A. *et al.* AMBER 2016. (University of California, San Francisco, 2016).
11. Jorgensen, W. L., Chandrasekhar, J., Madura, J. D., Impey, R. W. & Klein, M. L. Comparison of Simple Potential Functions for Simulating Liquid Water. *J. Chem. Phys.* **79**, 926-935 (1983).
12. Joung, I. S. & Cheatham, T. E. Determination of alkali and halide monovalent ion parameters for use in explicitly solvated biomolecular simulations. *J. Phys. Chem. B* **112**, 9020-9041 (2008).
13. Li, P. F., Roberts, B. P., Chakravorty, D. K. & Merz, K. M. Rational design of particle mesh ewald compatible Lennard-Jones parameters for +2 metal cations in explicit solvent. *J. Chem. Theory Comput.* **9**, 2733-2748 (2013).
14. Gohlke, H., Kiel, C. & Case, D. A. Insights into protein-protein binding by binding free energy calculation and free energy decomposition for the Ras-Raf and Ras-RaIGDS complexes. *J. Mol. Biol.* **330**, 891-913 (2003).
